# Supplementary material for: Function-on-Scalar Quantile Regression with Application to Mass Spectrometry Proteomics Data
Source: arXiv:1809.00266 source file (2019-10-03)
Supplement: Supplementary file 1 [file supplementary_arxiv.pdf]

# Function-on-Scalar Quantile Regression with Application to Mass Spectrometry Proteomics Data: Supplementary Materials

Yusha Liu<sup>\*</sup>, Meng Li<sup>\*</sup> and Jeffrey S. Morris<sup>†</sup>

*<sup>\*</sup>Department of Statistics, Rice University*

*<sup>†</sup>Department of Biostatistics, University of Texas MD Anderson Cancer Center*

August 31, 2018

This document includes mathematical details of the MCMC sampling procedure, additional results of mass spectrometry data application, and implementation details of FDboost package.

# 1 Posterior computation via MCMC sampling

## 1.1 Detailed Gibbs sampling procedures for horseshor prior on basis coefficients

We detail the Gibbs sampling procedures to draw posterior samples of the parameters in model (4) in the main paper from their full conditional posterior distributions. We describe how to update the global and local shrinkage parameters if a horseshoe prior is placed on  $B_{ajh}^*$ , which is used in simulation studies and real data application in this paper. Specifically, it is assumed that  $\lambda_{ajh} \sim C^+(0, 1)$  and  $\psi_{aj} \sim C^+(0, s_a)$ , where  $s_a$  can either be fixed as 1 (Carvalho et al., 2009), or treated as a hyperparameter and given a vague hyperprior. Here we choose to assign  $s_a^2$  a vague inverse Gamma hyperprior with a mode of 1. To update  $\lambda_{ajh}$  and  $\psi_{aj}$ , we make use of the inverse Gamma scale mixture representation for the half Cauchy distribution (Makalic and Schmidt, 2016) and introduce the auxiliary variables  $\nu_{ajh}$  and  $\gamma_{aj}$ , i.e.,

$$\begin{aligned}\lambda_{ajh}^2 | \nu_{ajh} &\sim \text{inverse Gamma} \left( \frac{1}{2}, \frac{1}{\nu_{ajh}} \right), & \nu_{ajh} &\sim \text{inverse Gamma} \left( \frac{1}{2}, 1 \right); \\ \psi_{aj}^2 | \gamma_{aj} &\sim \text{inverse Gamma} \left( \frac{1}{2}, \frac{1}{\gamma_{aj}} \right), & \gamma_{aj} &\sim \text{inverse Gamma} \left( \frac{1}{2}, \frac{1}{s_a^2} \right).\end{aligned}$$

The parameters to be updated are  $\{B_a(t_l)\}$ ,  $\{\sigma(t_l)\}$ ,  $\{\xi_i(t_l)\}$ ,  $\{B_{ajh}^*\}$ ,  $\{\lambda_{ajh}\}$ ,  $\{\nu_{ajh}\}$ ,  $\{\psi_{aj}\}$ ,  $\{\gamma_{aj}\}$  and  $\{s_a\}$ . For initialization, we compute the initial values of  $B_a(t)$  in model (1) in the main paper by obtaining their maximum likelihood estimates (MLE) assuming *i.i.d.* Gaussian errors for  $E_i(t)$ , and initialize  $\mathbf{B}^*$  using  $\mathbf{B}^* = \mathbf{B}\Phi^-$ , where  $\Phi^- = \Phi'(\Phi\Phi')^{-1}$  is the Moore-Penrose generalized inverse matrix of  $\Phi$  in equation (5) in the main paper. The initial value of  $s_a$  is set to 1, and the initial values of  $\lambda_{ajh}$ ,  $\nu_{ajh}$ ,  $\psi_{aj}$  and  $\gamma_{aj}$  are obtained by sampling from their prior distributions respectively. Below are the steps of posterior sampling with derivation.

1. For each position  $l$ ,  $\sigma(t_l)$  has a vague prior of inverse Gamma  $(\alpha_{\sigma_l}, \beta_{\sigma_l})$ . Update  $\sigma(t_l)$  by  $(\sigma(t_l) \mid \mathbf{B}(t_l), \mathbf{y}(t_l), \alpha_{\sigma_l}, \beta_{\sigma_l}) \sim \text{inverse Gamma} \left( N + \alpha_{\sigma_l}, \sum_{i=1}^N \rho_{\tau} (Y_i(t_l) - \mathbf{X}_i' \mathbf{B}(t_l)) + \beta_{\sigma_l} \right)$ . Note that the conditional distributions of  $\sigma(t_l)$  are obtained by integrating out latent variables  $\xi_i(t_l)$ , leading to a partially collapsed Gibbs step with improved mixing properties.

2. For each subject  $i$  and position  $l$ , update  $\xi_i(t_l)$  by  $(1/\xi_i(t_l) \mid \mathbf{B}(t_l), Y_i(t_l), \sigma(t_l)) \sim \text{inverse Gaussian}(1/\{\tau(1-\tau) \mid Y_i(t_l) - \mathbf{X}'_i \mathbf{B}(t_l)\}, 1/\{2\tau(1-\tau)\sigma(t_l)\})$ .
3. For each covariate  $a$ , update  $\mathbf{B}_a^*$  from  $f(\mathbf{B}_a^* \mid \mathbf{B}_{-a}^*, \mathbf{Y}, \boldsymbol{\sigma}, \boldsymbol{\xi}, \boldsymbol{\lambda}_a, \boldsymbol{\psi}_a)$ , where  $\mathbf{B}_{-a}^*$  is the  $(p-1) \times K$  matrix of basis coefficients with the  $a^{\text{th}}$  row excluded from  $\mathbf{B}^*$ ,  $\boldsymbol{\xi}$  is the  $N \times T$  matrix of latent variables with  $\boldsymbol{\xi}(i, l) = \xi_i(t_l)$ ,  $\boldsymbol{\sigma} = \{\sigma(t_l)\}_l$ ,  $\boldsymbol{\lambda}_a = \{\lambda_{ajh}\}_{j,h}$ ,  $\boldsymbol{\psi}_a = \{\psi_{aj}\}_j$ . Projection of  $\mathbf{B}$  into the basis space is performed in this step, which can be computed by  $\mathbf{B}^* = \mathbf{B}\Phi^-$ . It turns out that

$$(\mathbf{B}_a^* \mid \mathbf{Y}, \mathbf{B}_{-a}^*, \boldsymbol{\sigma}, \boldsymbol{\xi}, \boldsymbol{\lambda}_a, \boldsymbol{\psi}_a) \sim MVN(\mu_a, \Lambda_a),$$

for some  $\mu_a$  and  $\Lambda_a$  defined below.

We next elaborate the derivation of the full conditional distributions of  $\mathbf{B}^*$ . For each subject  $i$  and position  $l$ , let  $\tilde{Y}_i(t_l) = Y_i(t_l) - \frac{1-2\tau}{\tau(1-\tau)}\xi_i(t_l)$ , we can rewrite model (4) in the main paper as

$$\tilde{Y}_i(t_l) = \mathbf{X}'_i \mathbf{B}(t_l) + \varepsilon_i(t_l), \quad \varepsilon_i(t_l) \sim N\left(0, \frac{2\xi_i(t_l)\sigma(t_l)}{\tau(1-\tau)}\right),$$

or in matrix form,

$$\tilde{\mathbf{Y}} = \mathbf{X}\mathbf{B} + \boldsymbol{\varepsilon}, \quad \boldsymbol{\varepsilon}(t_l) \sim MVN(0, \boldsymbol{\Xi}_l),$$

where  $\boldsymbol{\Xi}_l = \text{diag}\left\{\frac{2\xi_i(t_l)\sigma(t_l)}{\tau(1-\tau)}\right\}_{i=1}^N$ . We rescale each column in the foregoing equation by premultiplying by  $\boldsymbol{\Xi}_l^{-\frac{1}{2}}$ , and obtain

$$\tilde{\mathbf{y}}_l^+ = \mathbf{X}_l^+ \mathbf{B}(t_l) + \boldsymbol{\varepsilon}_l^+, \quad \boldsymbol{\varepsilon}_l^+ \sim MVN(0, \mathbf{I}_N), \quad (1)$$

where  $\tilde{\mathbf{y}}_l^+ = \boldsymbol{\Xi}_l^{-\frac{1}{2}}\tilde{\mathbf{y}}(t_l)$ ,  $\mathbf{X}_l^+ = \boldsymbol{\Xi}_l^{-\frac{1}{2}}\mathbf{X}$ , and  $\boldsymbol{\varepsilon}_l^+ = \boldsymbol{\Xi}_l^{-\frac{1}{2}}\boldsymbol{\varepsilon}(t_l)$  are the rescaled versions of the responses, design matrix and residuals for position  $t_l$ . Let  $\tilde{\mathbf{y}}_l^{++} = \tilde{\mathbf{y}}_l^+ - \mathbf{X}_{(-a)l}^+ \mathbf{B}_{(-a)}(t_l)$ , where  $\mathbf{X}_{al}^+$  represents the  $a^{\text{th}}$  column of  $\mathbf{X}_l^+$  and  $\mathbf{X}_{(-a)l}^+$  is  $\mathbf{X}_l^+$  with the  $a^{\text{th}}$  column removed,  $\hat{B}_a(t_l) = \left(\mathbf{X}_{al}^{+'} \mathbf{X}_{al}^+\right)^{-1} \mathbf{X}_{al}^{+'} \tilde{\mathbf{y}}_l^{++}$ ,  $V_{al} = \left(\mathbf{X}_{al}^{+'} \mathbf{X}_{al}^+\right)^{-1}$ ,  $\hat{\mathbf{B}}_a = \left(\hat{B}_a(t_1), \dots, \hat{B}_a(t_T)\right)'$ ,  $\mathbf{V}_a = \text{diag}\{V_{al}\}_{l=1}^T$ ,  $\mathbf{v}_a = \text{diag}\{\lambda_{ajh}^2 \psi_{aj}^2\}_{j,h}$ ,  $\mathbf{B}_a^* = \Phi^{-'} \mathbf{B}_a$ ,  $\hat{\mathbf{B}}_a^* = \Phi^{-'} \hat{\mathbf{B}}_a$ , and  $\boldsymbol{\Sigma}_a = \Phi^{-'} \mathbf{V}_a \Phi^-$ . Note that  $\hat{B}_a(t_l)$  is the MLE of  $B_a(t_l)$  in model (1) conditional on  $\mathbf{B}_{-a}(t_l)$ , the scale parameter  $\sigma(t_l)$  and the latent variables  $\{\xi_i(t_l)\}_{i=1}^N$ ;  $V_{al}$  is the variance of this MLE. Assuming independent  $\boldsymbol{\varepsilon}_l^+$  across  $l$  as done in our model

and projecting into the basis space,  $\hat{\mathbf{B}}_a^*$  takes the form of MLE of  $\mathbf{B}_a^*$  conditional on  $\mathbf{B}_{-a}^*$  and scale parameters;  $\Sigma_a$  is the covariance matrix of  $\hat{\mathbf{B}}_a^*$ .

Then the conditional distributions of  $\mathbf{B}^*$  are obtained by

$$\begin{aligned}
& f(\mathbf{B}_a^* \mid \mathbf{Y}, \mathbf{B}_{-a}^*, \boldsymbol{\sigma}, \boldsymbol{\xi}, \boldsymbol{\lambda}_a, \boldsymbol{\psi}_a) \propto f(\mathbf{Y} \mid \mathbf{B}_a^*, \mathbf{B}_{-a}^*, \boldsymbol{\sigma}, \boldsymbol{\xi}) f(\mathbf{B}_a^* \mid \boldsymbol{\lambda}_a, \boldsymbol{\psi}_a) \\
& \propto \prod_{l=1}^T f(\mathbf{y}(t_l) \mid \mathbf{B}(t_l), \boldsymbol{\sigma}(t_l), \boldsymbol{\xi}(t_l)) f(\mathbf{B}_a^* \mid \boldsymbol{\lambda}_a, \boldsymbol{\psi}_a) \\
& \propto \prod_{l=1}^T \exp \left[ -\frac{1}{2} (\tilde{\mathbf{y}}_l^+ - \mathbf{X}_l^+ \mathbf{B}(t_l))' \mathbf{I}_N^{-1} (\tilde{\mathbf{y}}_l^+ - \mathbf{X}_l^+ \mathbf{B}(t_l)) \right] f(\mathbf{B}_a^* \mid \boldsymbol{\lambda}_a, \boldsymbol{\psi}_a) \\
& \propto \prod_{l=1}^T \exp \left[ -\frac{1}{2} (\tilde{\mathbf{y}}_l^{++} - \mathbf{X}_{al}^+ B_a(t_l))' (\tilde{\mathbf{y}}_l^{++} - \mathbf{X}_{al}^+ B_a(t_l)) \right] \prod_{j,h} f(B_{ajh}^* \mid \lambda_{ajh}, \psi_{aj}) \\
& \propto \prod_{l=1}^T \exp \left[ -\frac{1}{2} \frac{(B_a(t_l) - \hat{B}_a(t_l))^2}{V_{al}} \right] \prod_{j,h} \exp \left[ -\frac{1}{2} \frac{B_{ajh}^{*2}}{\lambda_{ajh}^2 \psi_{aj}^2} \right] \\
& \propto \exp \left[ -\frac{1}{2} (\mathbf{B}_a - \hat{\mathbf{B}}_a)' \mathbf{V}_a^{-1} (\mathbf{B}_a - \hat{\mathbf{B}}_a) \right] \exp \left[ -\frac{1}{2} \mathbf{B}_a^{*'} \mathbf{v}_a^{-1} \mathbf{B}_a^* \right] \\
& \propto \exp \left[ -\frac{1}{2} (\mathbf{B}_a^* - \hat{\mathbf{B}}_a^*)' \Sigma_a^{-1} (\mathbf{B}_a^* - \hat{\mathbf{B}}_a^*) \right] \exp \left[ -\frac{1}{2} \mathbf{B}_a^{*'} \mathbf{v}_a^{-1} \mathbf{B}_a^* \right] \\
& \propto \exp \left[ -\frac{1}{2} (\mathbf{B}_a^* - \boldsymbol{\mu}_a)' \boldsymbol{\Lambda}_a^{-1} (\mathbf{B}_a^* - \boldsymbol{\mu}_a) \right],
\end{aligned}$$

$\boldsymbol{\mu}_a = [\mathbf{I}_K - \Sigma_a \mathbf{v}_a^{-1} (\mathbf{I}_K + \Sigma_a \mathbf{v}_a^{-1})^{-1}] \hat{\mathbf{B}}_a^*$  and  $\boldsymbol{\Lambda}_a = [\mathbf{I}_K - \Sigma_a \mathbf{v}_a^{-1} (\mathbf{I}_K + \Sigma_a \mathbf{v}_a^{-1})^{-1}] \Sigma_a$ . The conditional mean  $\boldsymbol{\mu}_a$  of  $\mathbf{B}_a^*$  is a product of the unshrunk estimator  $\hat{\mathbf{B}}_a^*$  and the shrinkage factor  $\mathbf{I}_K - \Sigma_a \mathbf{v}_a^{-1} (\mathbf{I}_K + \Sigma_a \mathbf{v}_a^{-1})^{-1}$ , which includes the regularization parameters through  $\mathbf{v}_a$ . Similarly, the conditional covariance matrix  $\boldsymbol{\Lambda}_a$  of  $\mathbf{B}_a^*$  is a product of this shrinkage factor and the unshrunk estimator  $\Sigma_a$ .

4. The updates of  $\lambda_{ajh}, \nu_{ajh}, \psi_{aj}, \gamma_{aj}$  follow the standard procedures for the horseshoe prior. For each covariate  $a$  and basis index  $j, h$ , update  $\lambda_{ajh}^2$  and  $\nu_{ajh}$  by

$$\begin{aligned}
(\lambda_{ajh}^2 \mid B_{ajh}^*, \nu_{ajh}, \psi_{aj}) & \sim \text{inverse Gamma} \left( 1, \frac{1}{2} \frac{B_{ajh}^{*2}}{\psi_{aj}^2} + \frac{1}{\nu_{ajh}} \right), \\
(\nu_{ajh} \mid \lambda_{ajh}) & \sim \text{inverse Gamma} \left( 1, \frac{1}{\lambda_{ajh}^2} + 1 \right).
\end{aligned}$$

For each covariate  $a$  and regularization subset  $j$ , update  $\psi_{aj}^2$  and  $\gamma_{aj}$  by

$$\begin{aligned} (\psi_{aj}^2 \mid \mathbf{B}_a^*, \boldsymbol{\lambda}_a, \gamma_{aj}) &\sim \text{inverse Gamma} \left( \frac{1}{2}H_j + \frac{1}{2}, \sum_{h=1}^{H_j} \frac{B_{ajh}^{*2}}{2\lambda_{ajh}^2} + \frac{1}{\gamma_{aj}} \right), \\ (\gamma_{aj} \mid \psi_{aj}^2, s_a) &\sim \text{inverse Gamma} \left( 1, \frac{1}{\psi_{aj}^2} + \frac{1}{s_a^2} \right). \end{aligned}$$

For each covariate  $a$ , the hyperparameter  $s_a^2$  has a vague hyperprior of inverse Gamma  $(\alpha_{s_a^2}, \beta_{s_a^2})$  with the mode at 1. Update  $s_a^2$  by

$$(s_a^2 \mid \boldsymbol{\gamma}_a, \alpha_{s_a^2}, \beta_{s_a^2}) \sim \text{inverse Gamma} \left( \frac{J}{2} + \alpha_{s_a^2}, \sum_{j=1}^J \frac{1}{\gamma_{aj}} + \beta_{s_a^2} \right).$$

5. Update  $\mathbf{B}$  by  $\mathbf{B} = \mathbf{B}^* \boldsymbol{\Phi}$ .

## 1.2 Other global-local shrinkage priors on basis coefficients

It is straightforward to modify the sampling step 4 in Section 1.1 to accommodate other computationally tractable global-local shrinkage priors, including the Gaussian prior, Laplace prior, Normal-Gamma Prior (Griffin et al., 2010), and Dirichlet-Laplace prior (Bhattacharya et al., 2015).

## 2 Extra results of application to pancreatic cancer dataset

At each quantile level, we examined the trace plots and autocorrelation plots of the posterior samples for various model parameters, which suggest good mixing of MCMC chains. Figure S1 and Figure S2 display the trace plots of the MCMC samples respectively for  $B_2^\tau(t_l)$  and  $\sigma^\tau(t_l)$  ( $\tau = 0.1, 0.25, 0.5, 0.75, 0.9$ ), at 16 spectral locations indexed by the evenly spaced vector  $l = 100, 200, \dots, 1600$ . We also conducted Geweke tests to perform a formal convergence check on model parameters. Figure S3 demonstrates the distributions of the p-values from Geweke tests on  $B_2^\tau(t_l)$  and  $\sigma^\tau(t_l)$  for all the location indices  $l = 1, 2, \dots, 1659$ , which do not suggest a violation of the null distribution  $Unif(0, 1)$  in each case. The proportions of p-values that are smaller than 0.05 are 0.058, 0.058, 0.061, 0.053, 0.059 respectively for  $\tau = 0.1, 0.25, 0.5, 0.75, 0.9$ .

The mean estimates of  $B_2^\tau(t)$  ( $\tau = 0.1, 0.25, 0.5, 0.75, 0.9$ ) and the corresponding 95% pointwise and simultaneous bands calculated from each approach are provided in Figure S4. A spectral location is flagged as significant if its SimBaS is less than or equal to 0.05 and its posterior estimate is greater than  $\frac{1}{2} \log_2(1.5)$  in magnitude (corresponding to at least a 1.5-fold change and indicated by two horizontal lines in Figure S4), and is marked by a vertical line on the x-axis in the corresponding plot. For each approach, the mean estimate of  $B_2^\tau(t)$  and identified locations differ greatly across quantiles. At  $\tau = 0.1, 0.25, 0.5$ , none of the approaches identify any location as significant; at  $\tau = 0.75, 0.9$ , certain locations are flagged by at least one approach. These comparisons across quantiles suggest that functional mean regression assuming a Gaussian distribution for the expression levels of a given protein within the same group could miss out on important proteomic differences between the cancer and normal cohorts, and functional quantile regression is strongly warranted in this case.

Comparing across methods at a given quantile, the two naïve approaches produce very wiggly estimate of  $B_2^\tau(t)$ , while the two-step bootstrap-based approaches appear to over-smooth the separate peaks in  $B_2^\tau(t)$  that are recognized by the Bayesian FQR model into one single broader peak. The Bayesian FQR model consistently produces substantially tighter 95% simultaneous band than the alternatives, among which the naïve bootstrap-based QR always results in the widest simultaneous band. At  $\tau = 0.75, 0.9$ , the naïve Bayesian QR and our proposed model flag essentially the same set of spectral locations as significantly different between the cancer and normal populations; the two-step bootstrap-based methods are able to identify most of these locations and the naïve bootstrap-based QR nearly miss all of them.

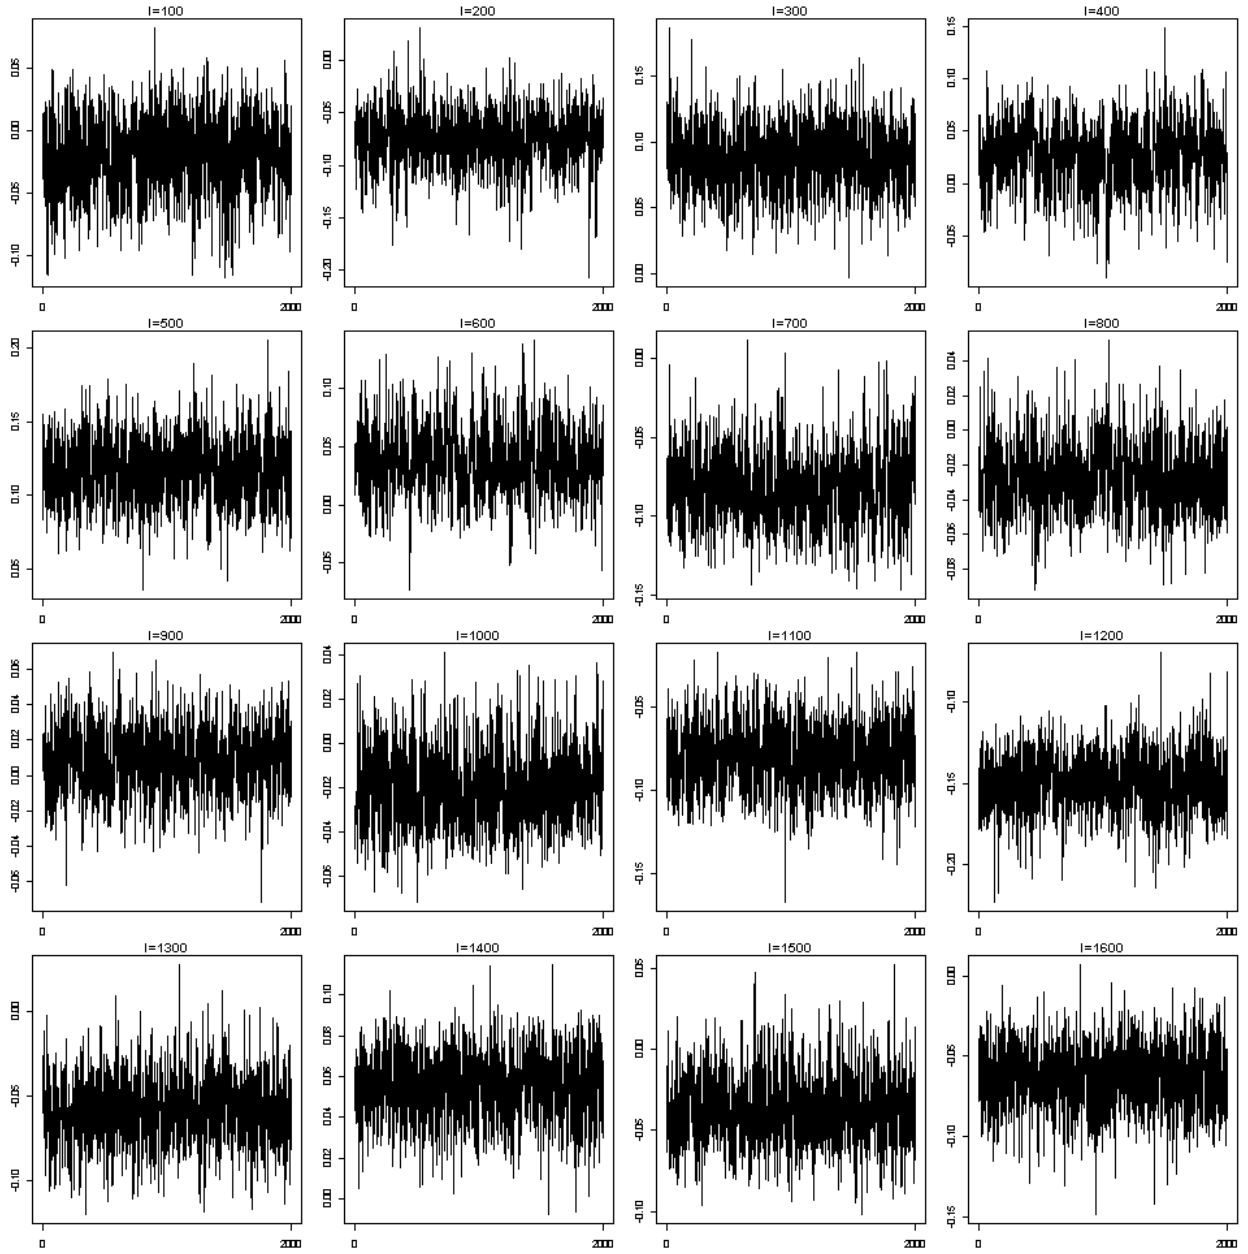

Figure S1(a): Trace plots of  $B_2^{0.1}(t_l)$  in the pancreatic cancer dataset for a chosen subset of location indices  $l$ .

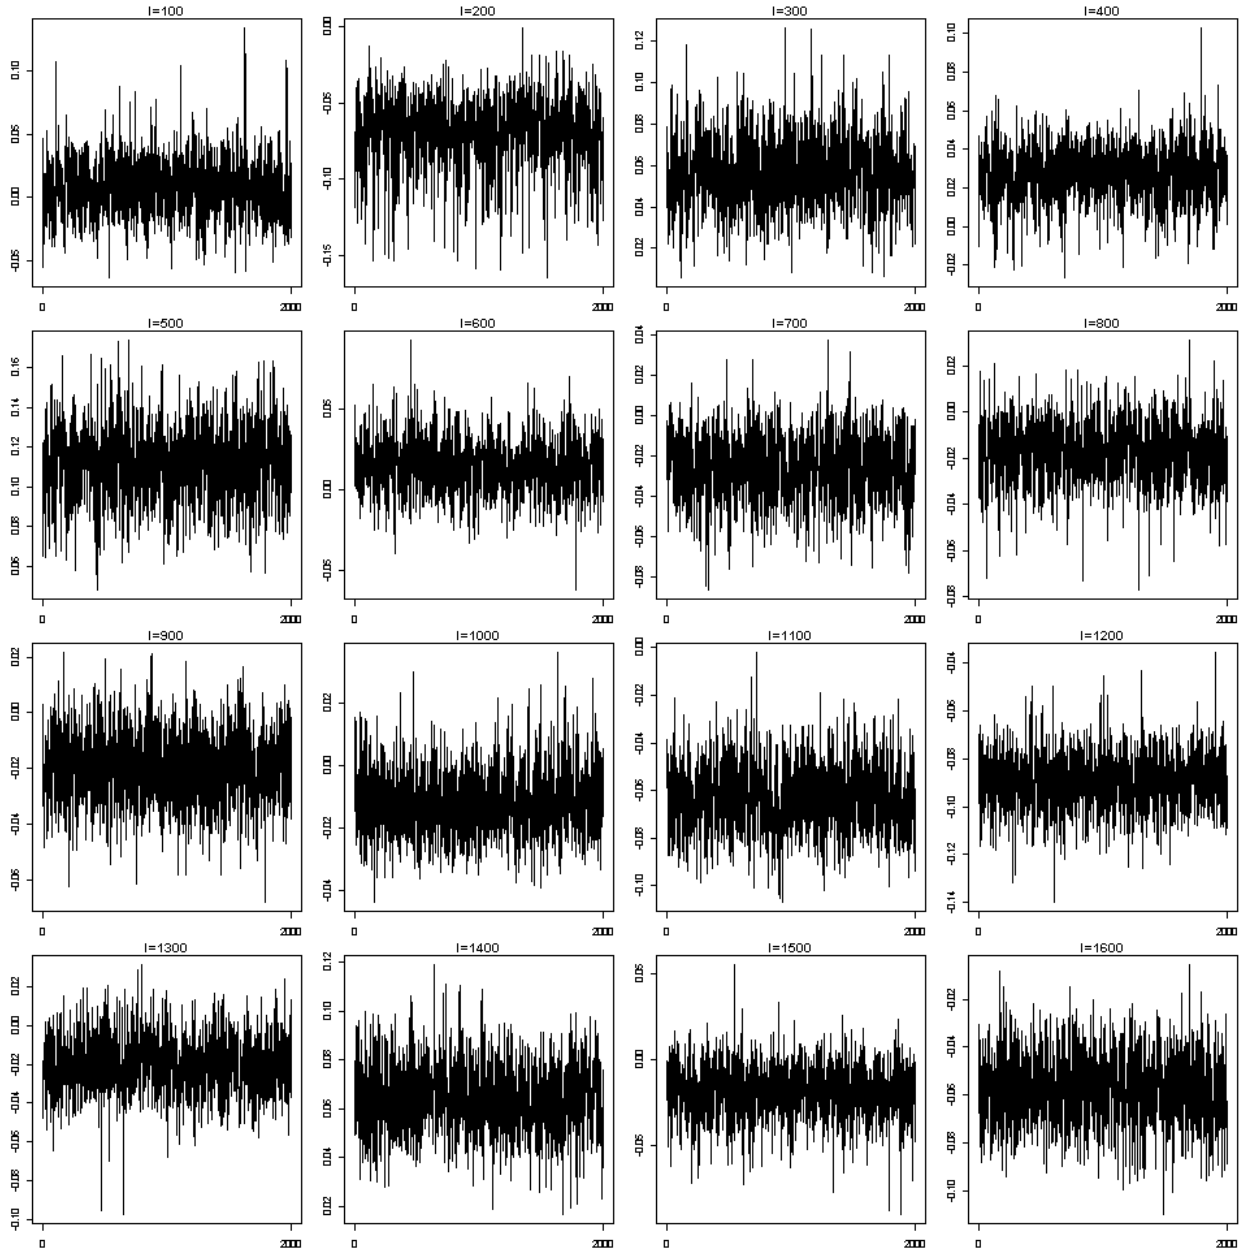

Figure S1(b): Trace plots of  $B_2^{0.25}(t_l)$  in the pancreatic cancer dataset for a chosen subset of location indices  $l$ .

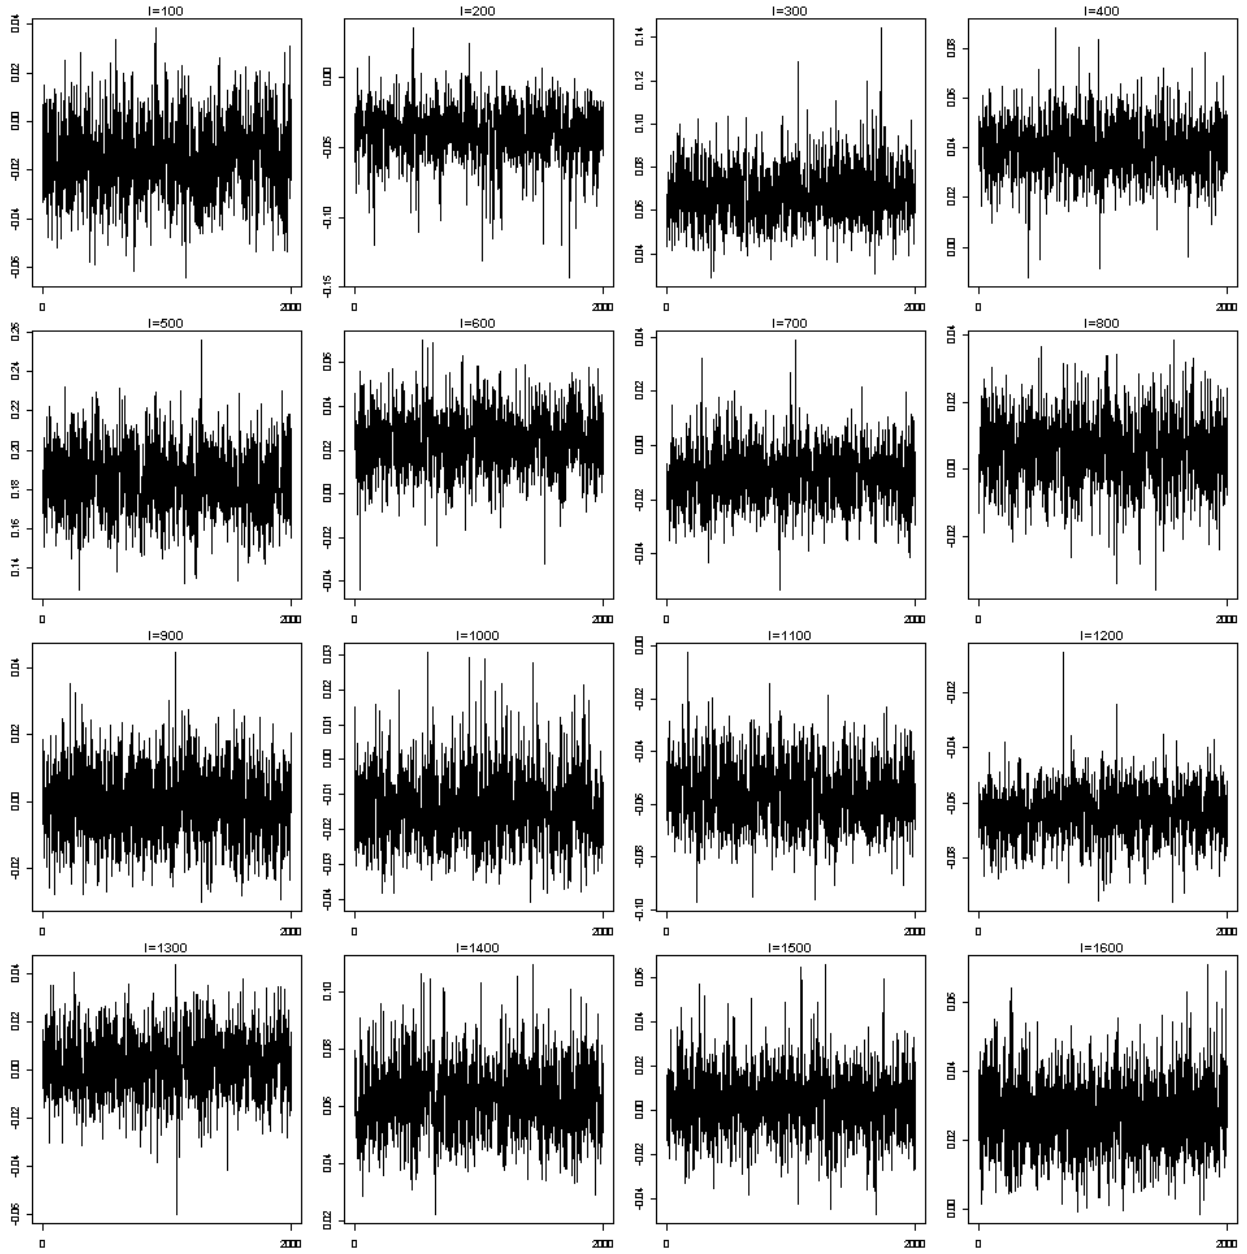

Figure S1(c): Trace plots of  $B_2^{0.5}(t_l)$  in the pancreatic cancer dataset for a chosen subset of location indices  $l$ .

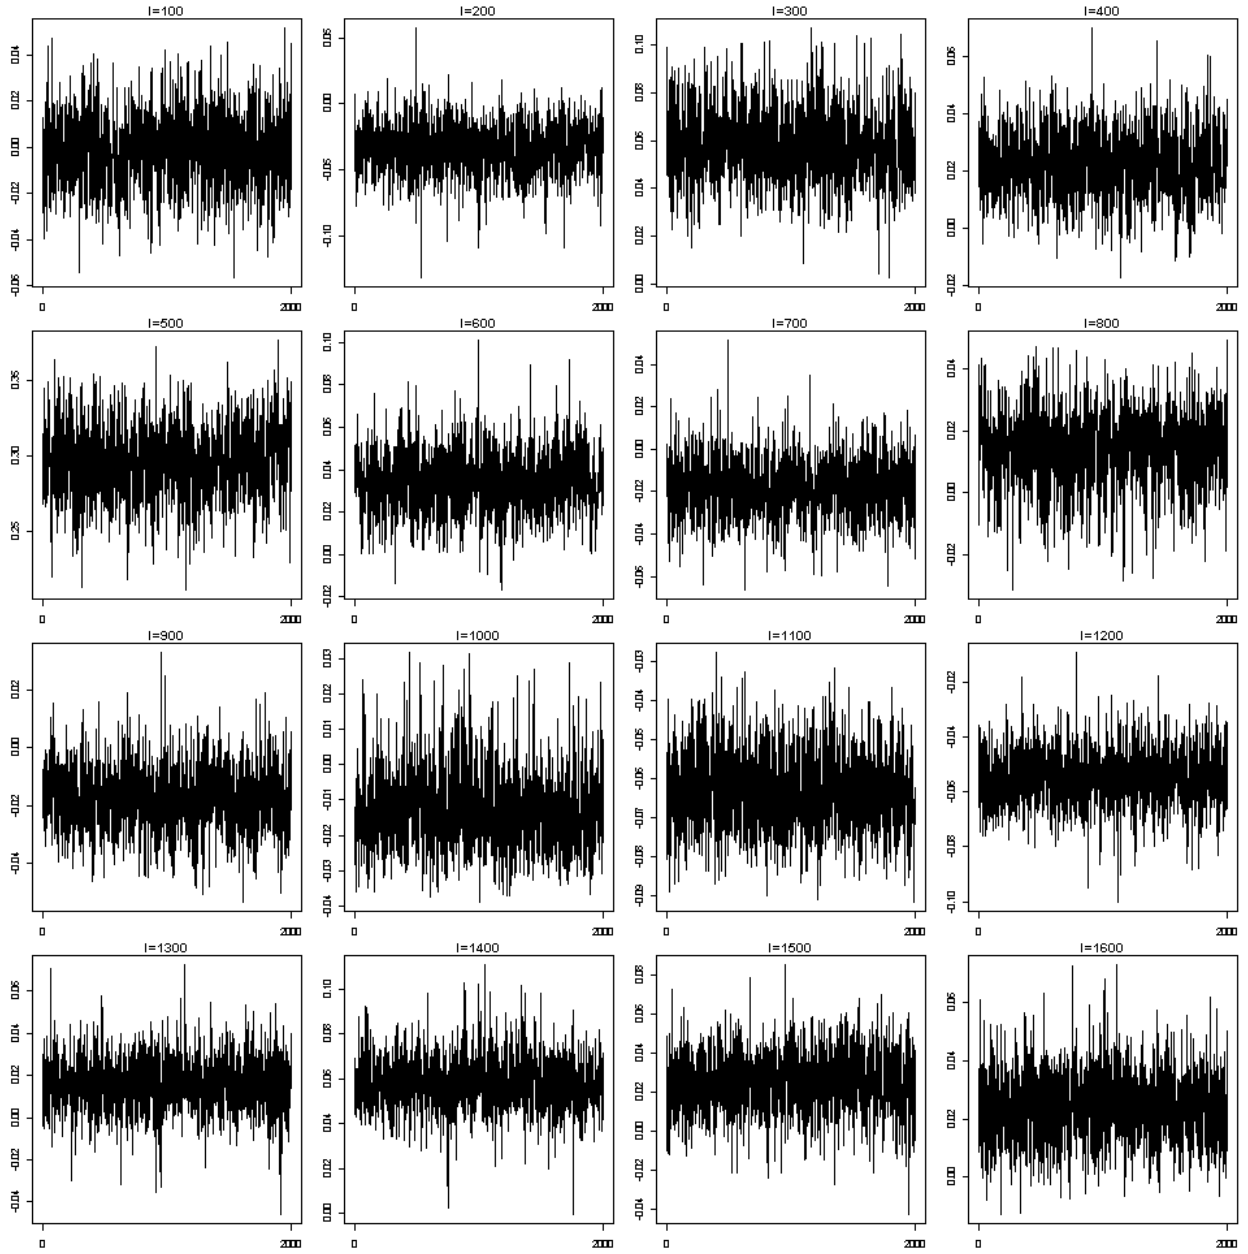

Figure S1(d): Trace plots of  $B_2^{0.75}(t_l)$  in the pancreatic cancer dataset for a chosen subset of location indices  $l$ .

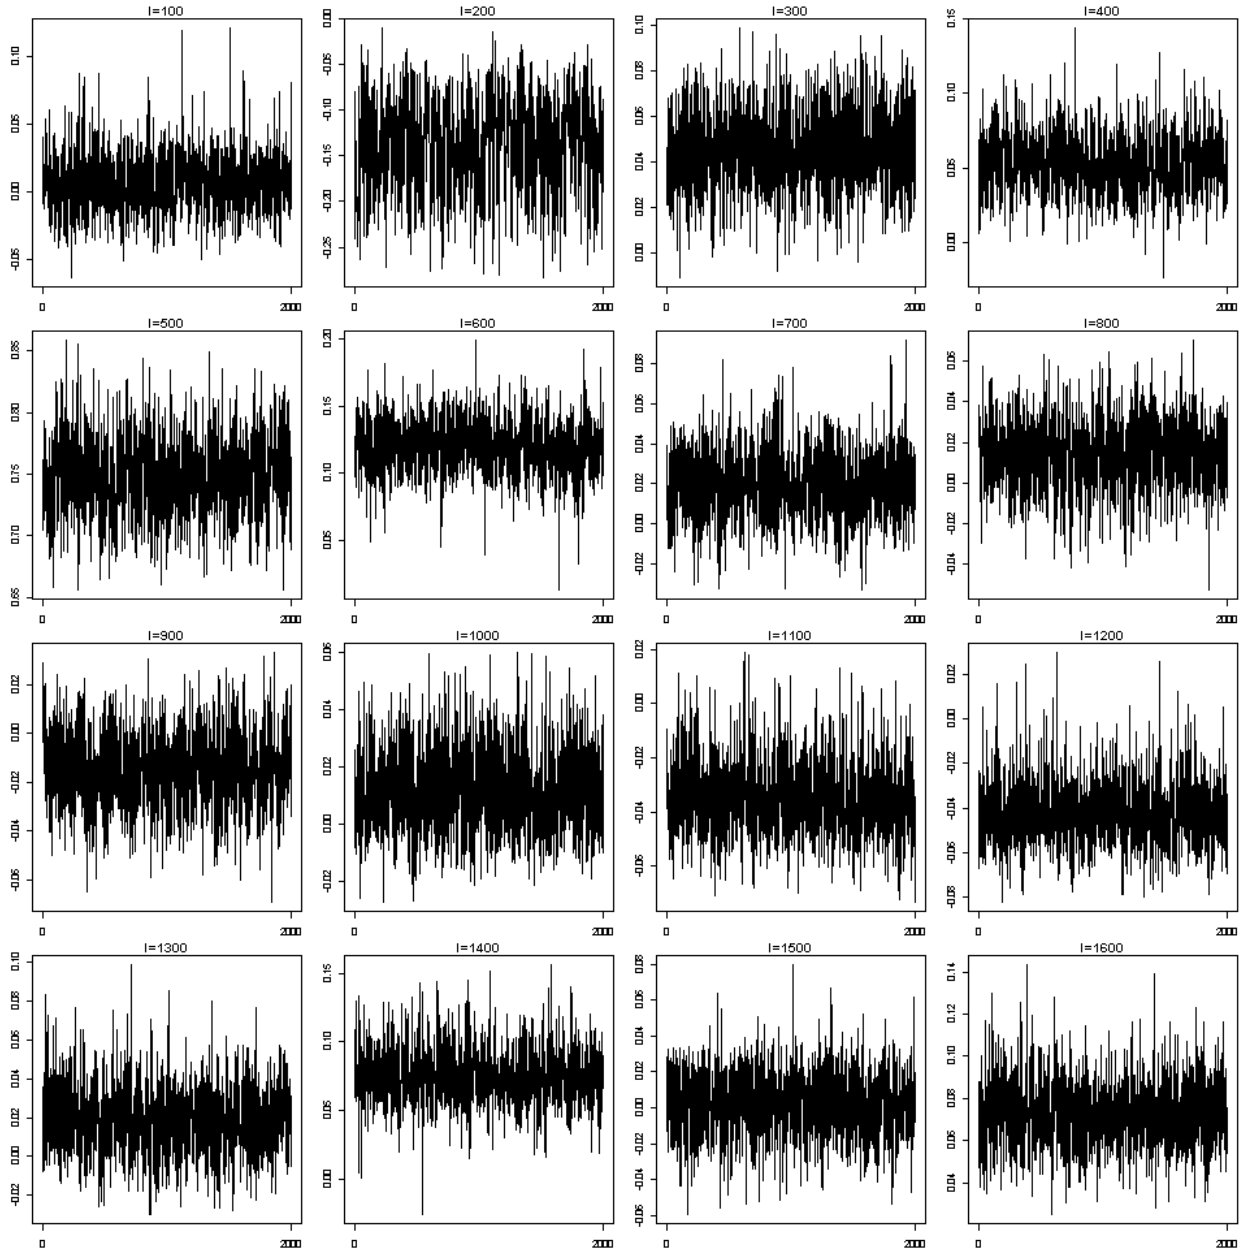

Figure S1(e): Trace plots of  $B_2^{0.9}(t_l)$  in the pancreatic cancer dataset for a chosen subset of location indices  $l$ .

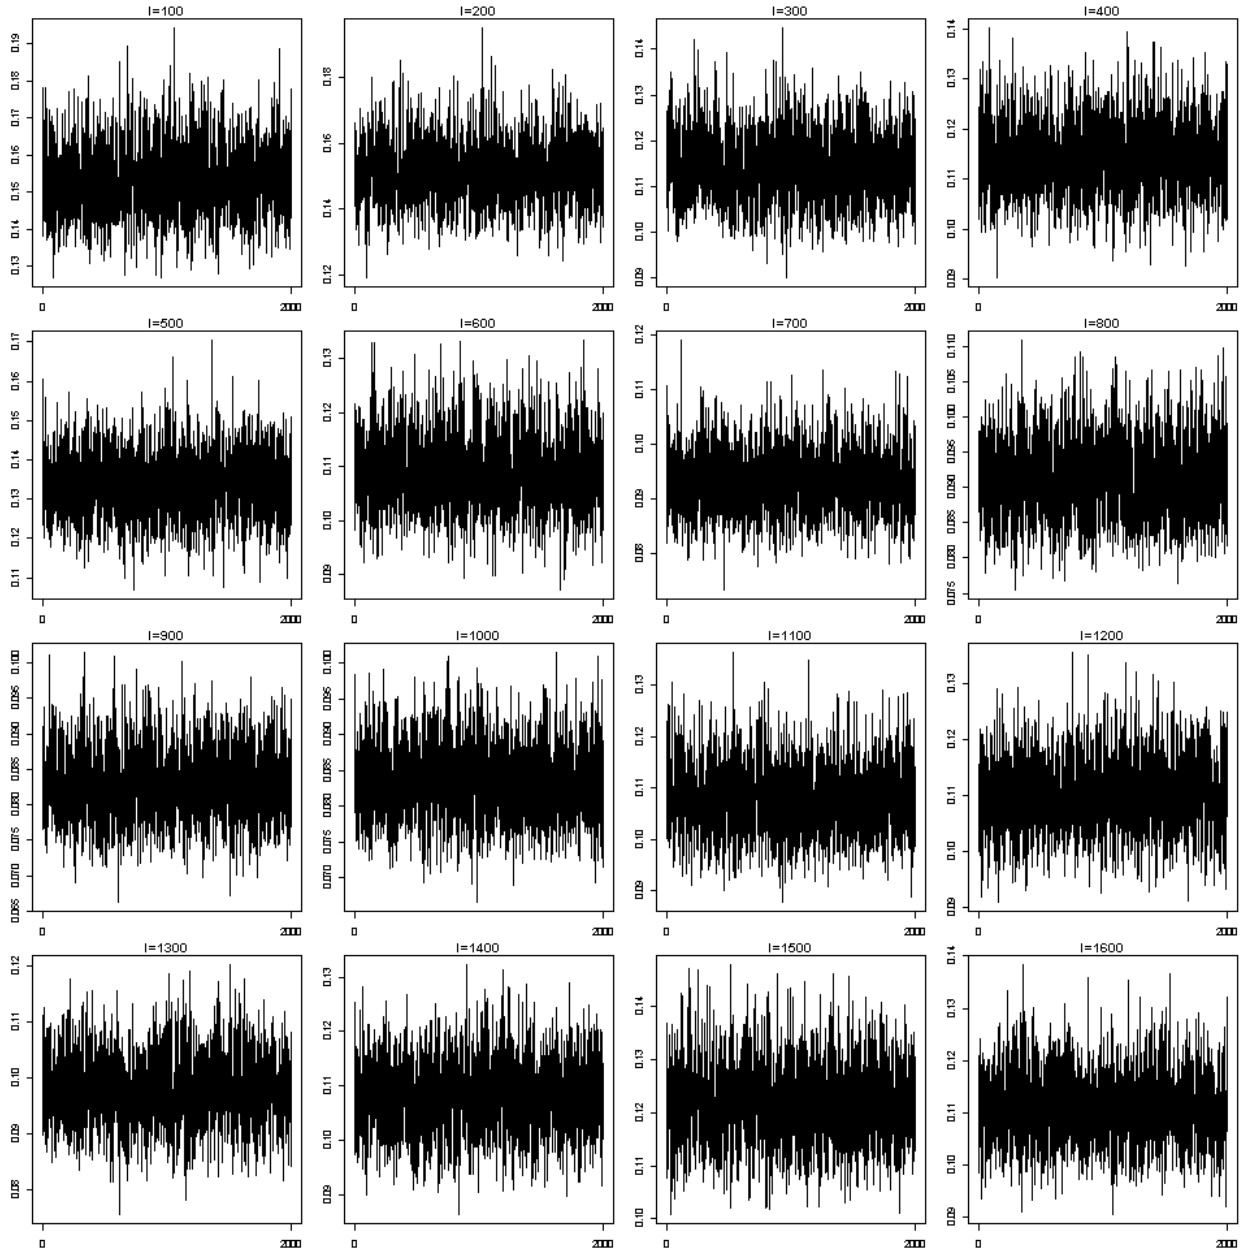

Figure S2(a): Trace plots of  $\sigma^{0.1}(t_l)$  in the pancreatic cancer dataset for a chosen subset of location indices  $l$ .

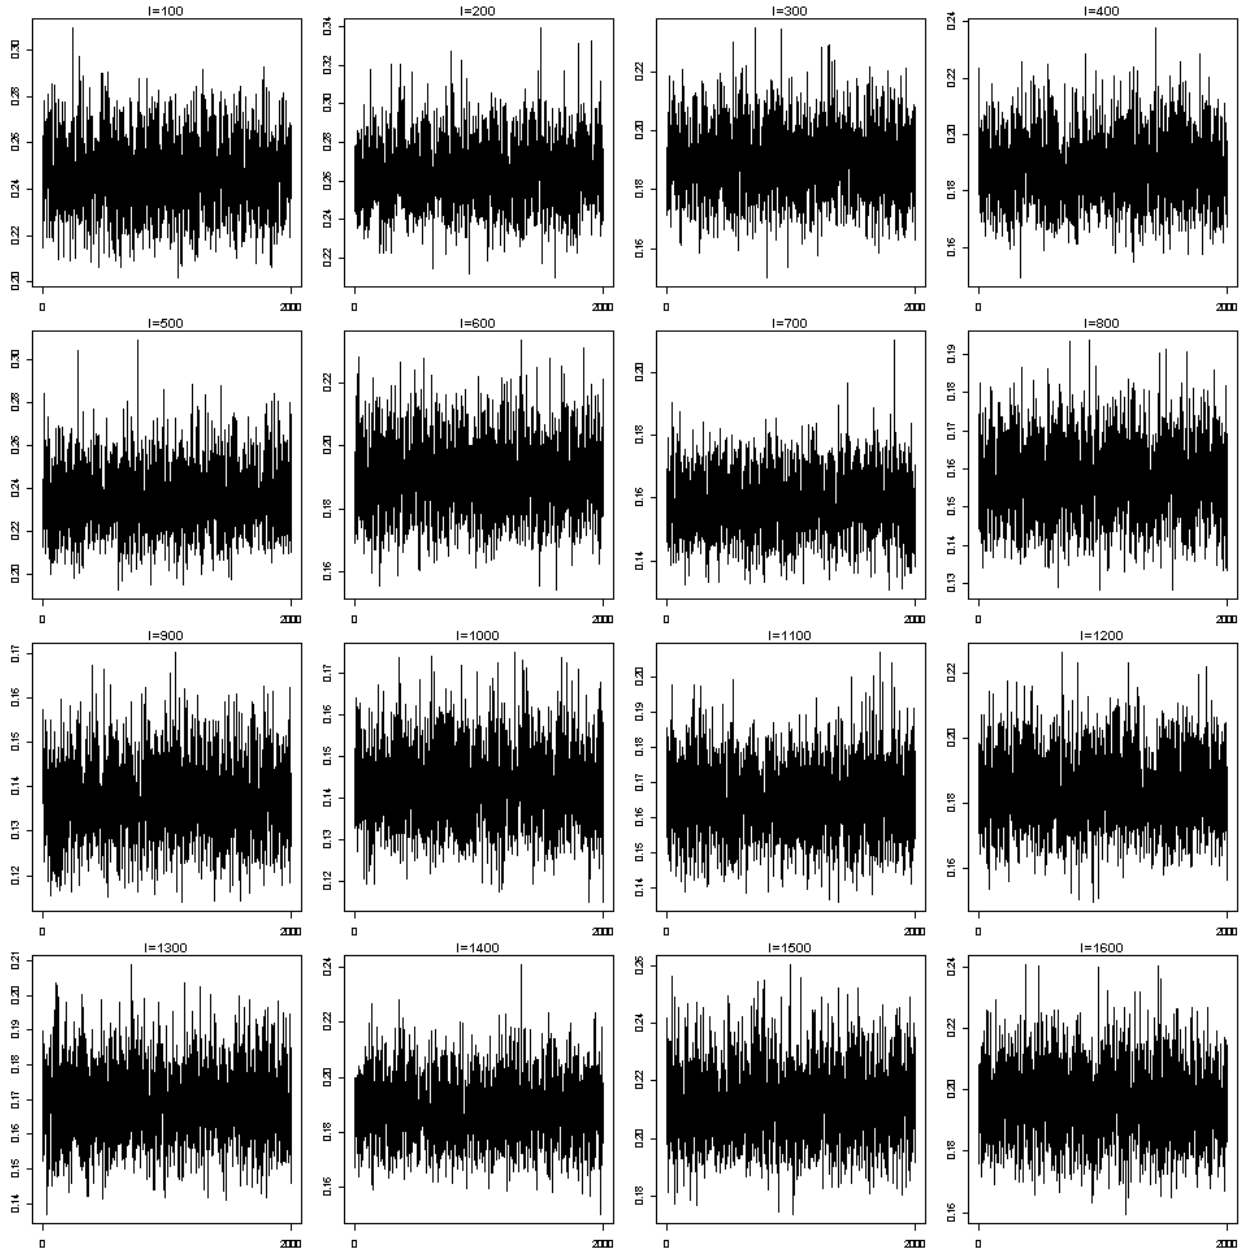

Figure S2(b): Trace plots of  $\sigma^{0.25}(t_l)$  in the pancreatic cancer dataset for a chosen subset of location indices  $l$ .

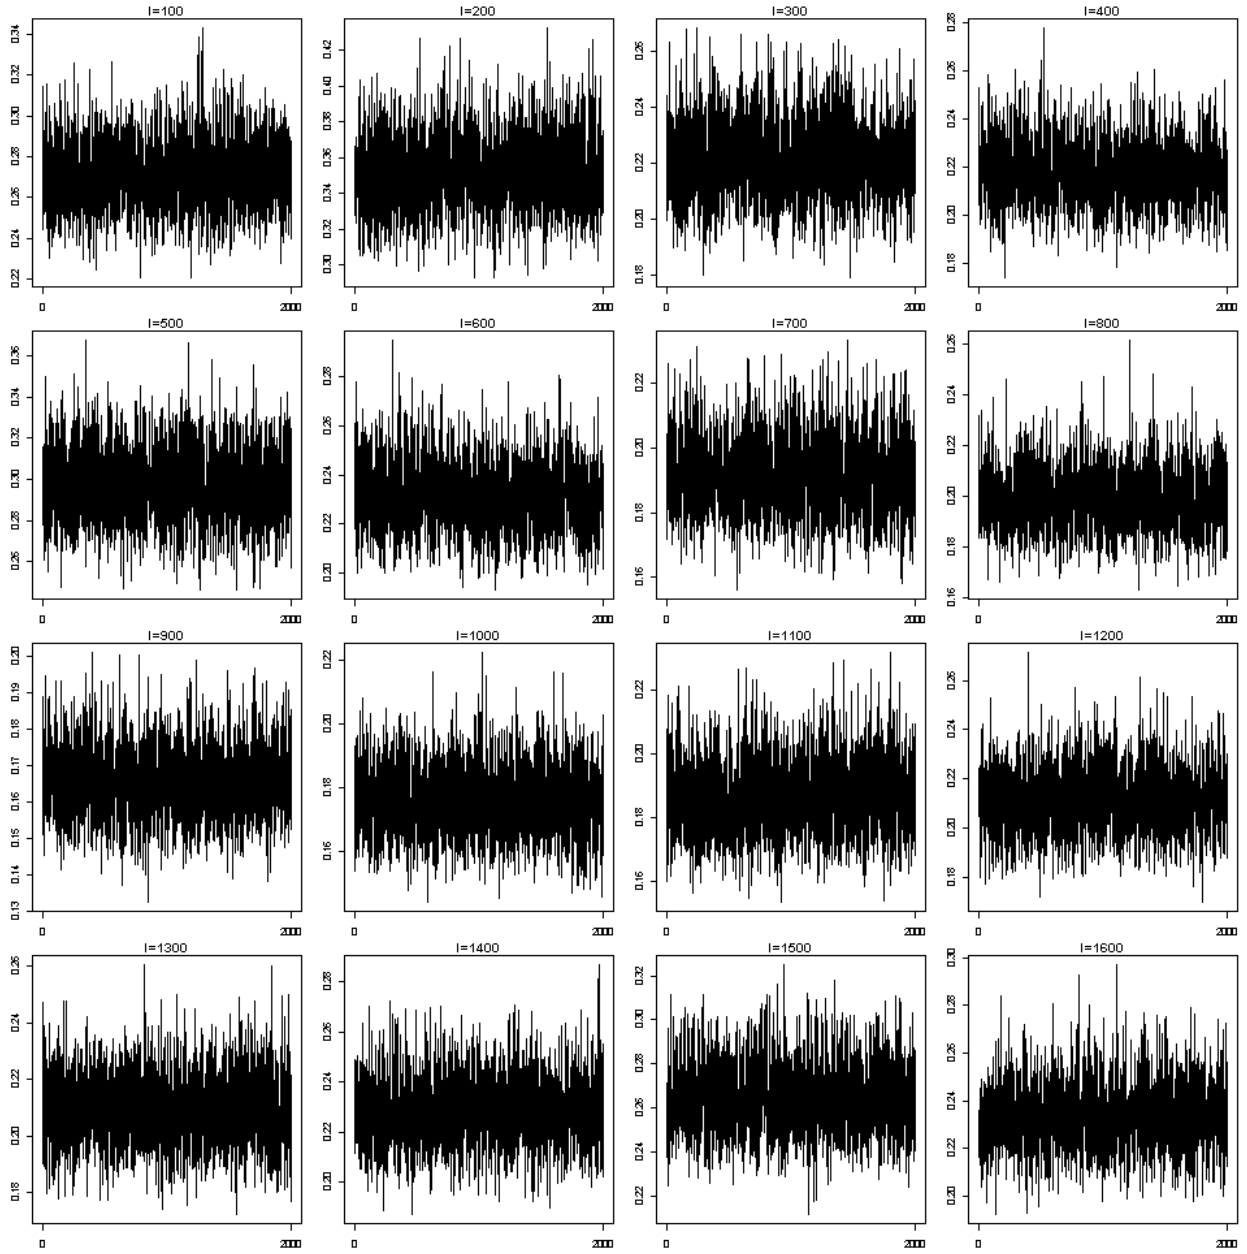

Figure S2(c): Trace plots of  $\sigma^{0.5}(t_l)$  in the pancreatic cancer dataset for a chosen subset of location indices  $l$ .

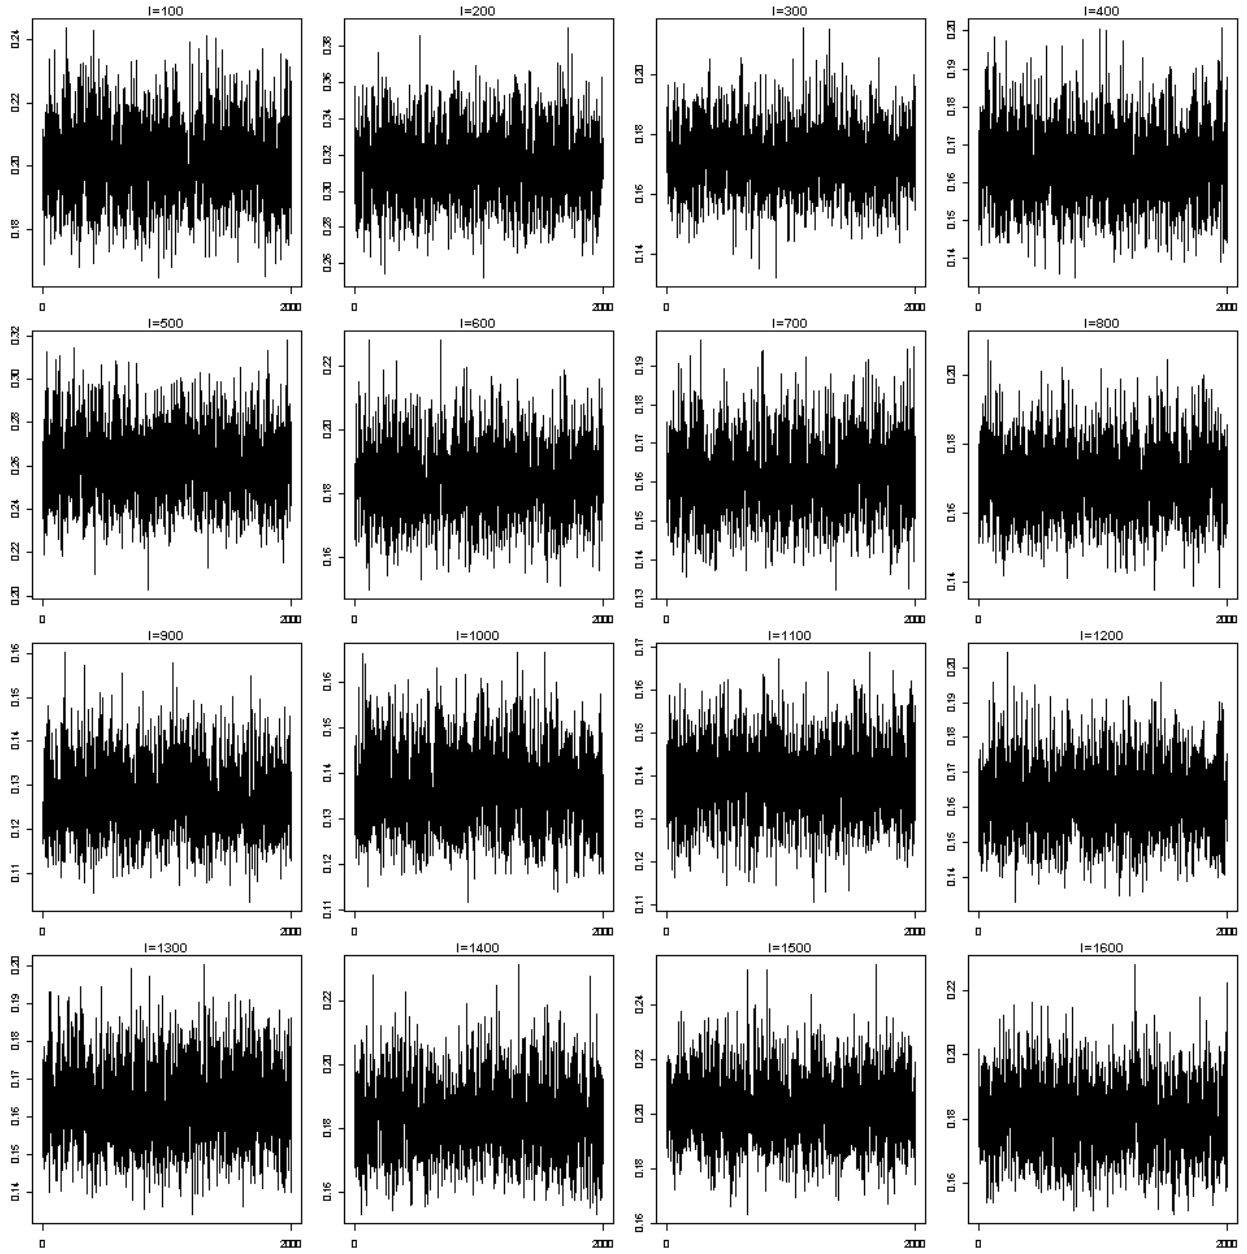

Figure S2(d): Trace plots of  $\sigma^{0.75}(t_l)$  in the pancreatic cancer dataset for a chosen subset of location indices  $l$ .

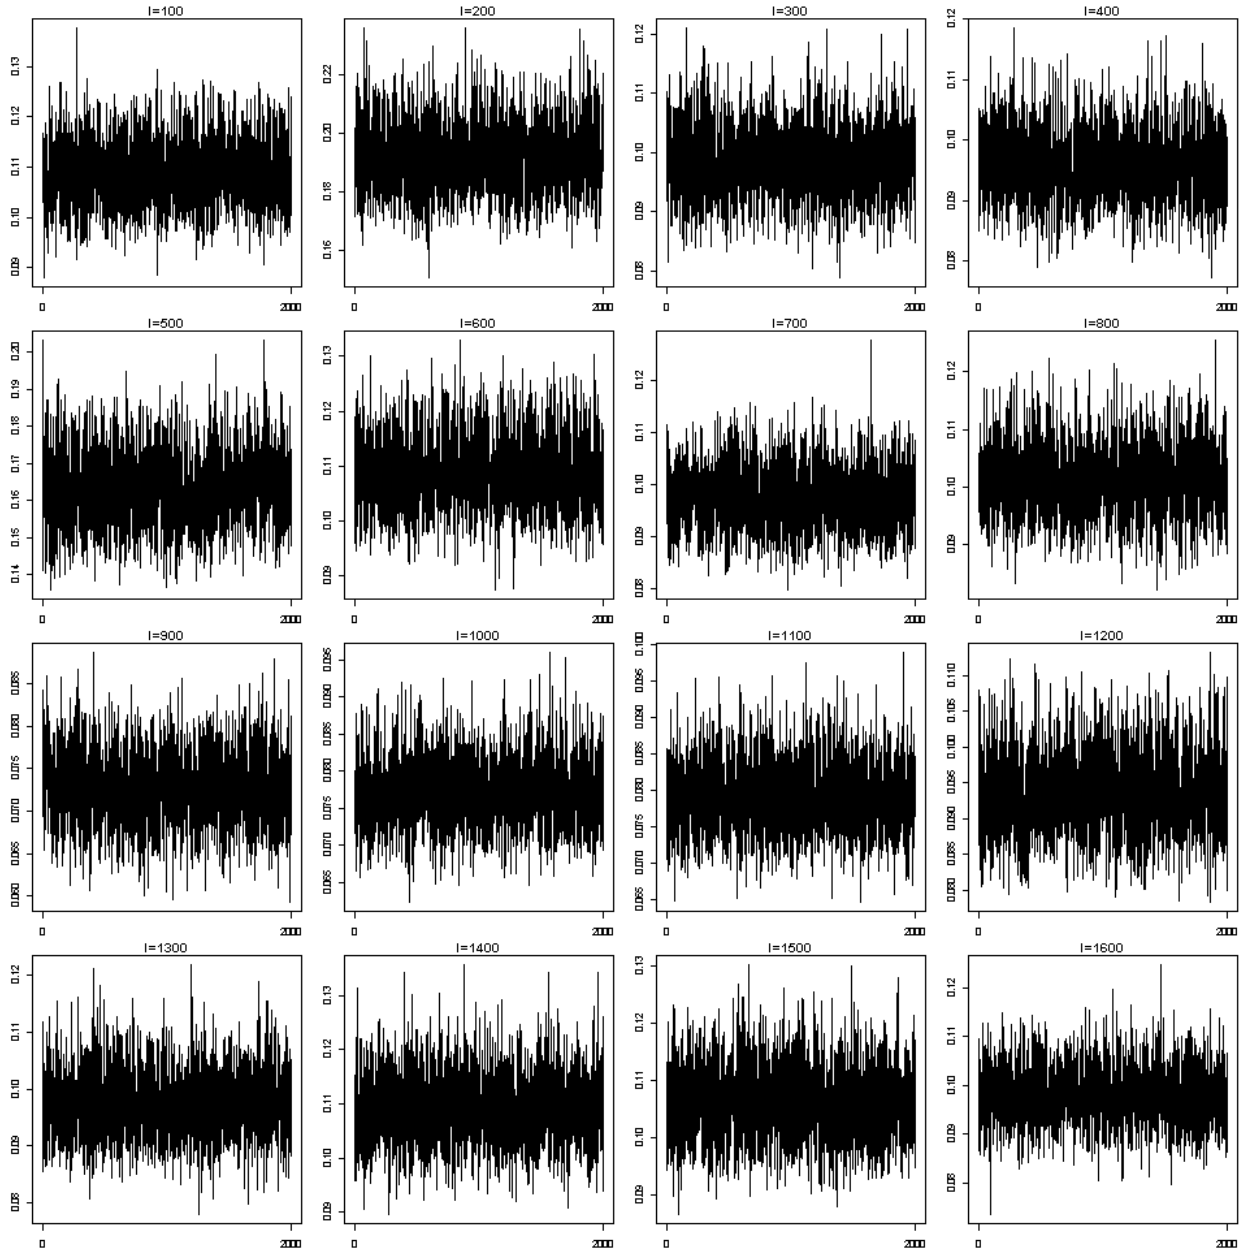

Figure S2(e): Trace plots of  $\sigma^{0.9}(t_l)$  in the pancreatic cancer dataset for a chosen subset of location indices  $l$ .

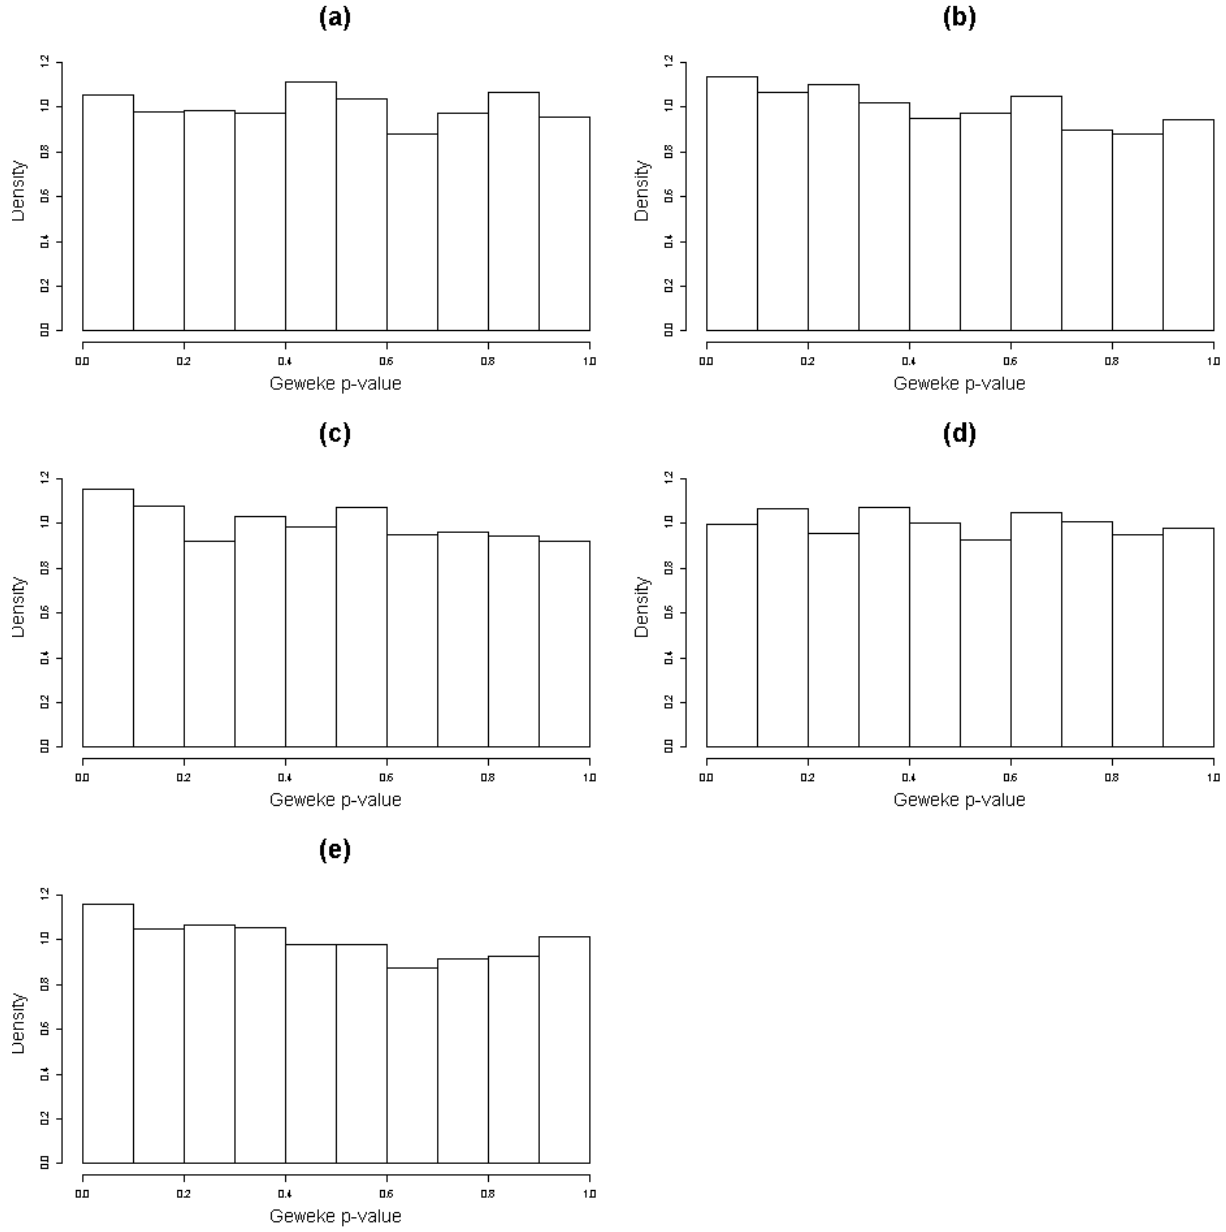

Figure S3: Distribution of p-values from Geweke tests on  $B_2^T(t_l)$  and  $\sigma^\tau(t_l)$  for all location indices  $l$  in the pancreatic cancer dataset, respectively for (a)  $\tau = 0.1$ , (b)  $\tau = 0.25$ , (c)  $\tau = 0.5$ , (d)  $\tau = 0.75$ , (e)  $\tau = 0.9$ .

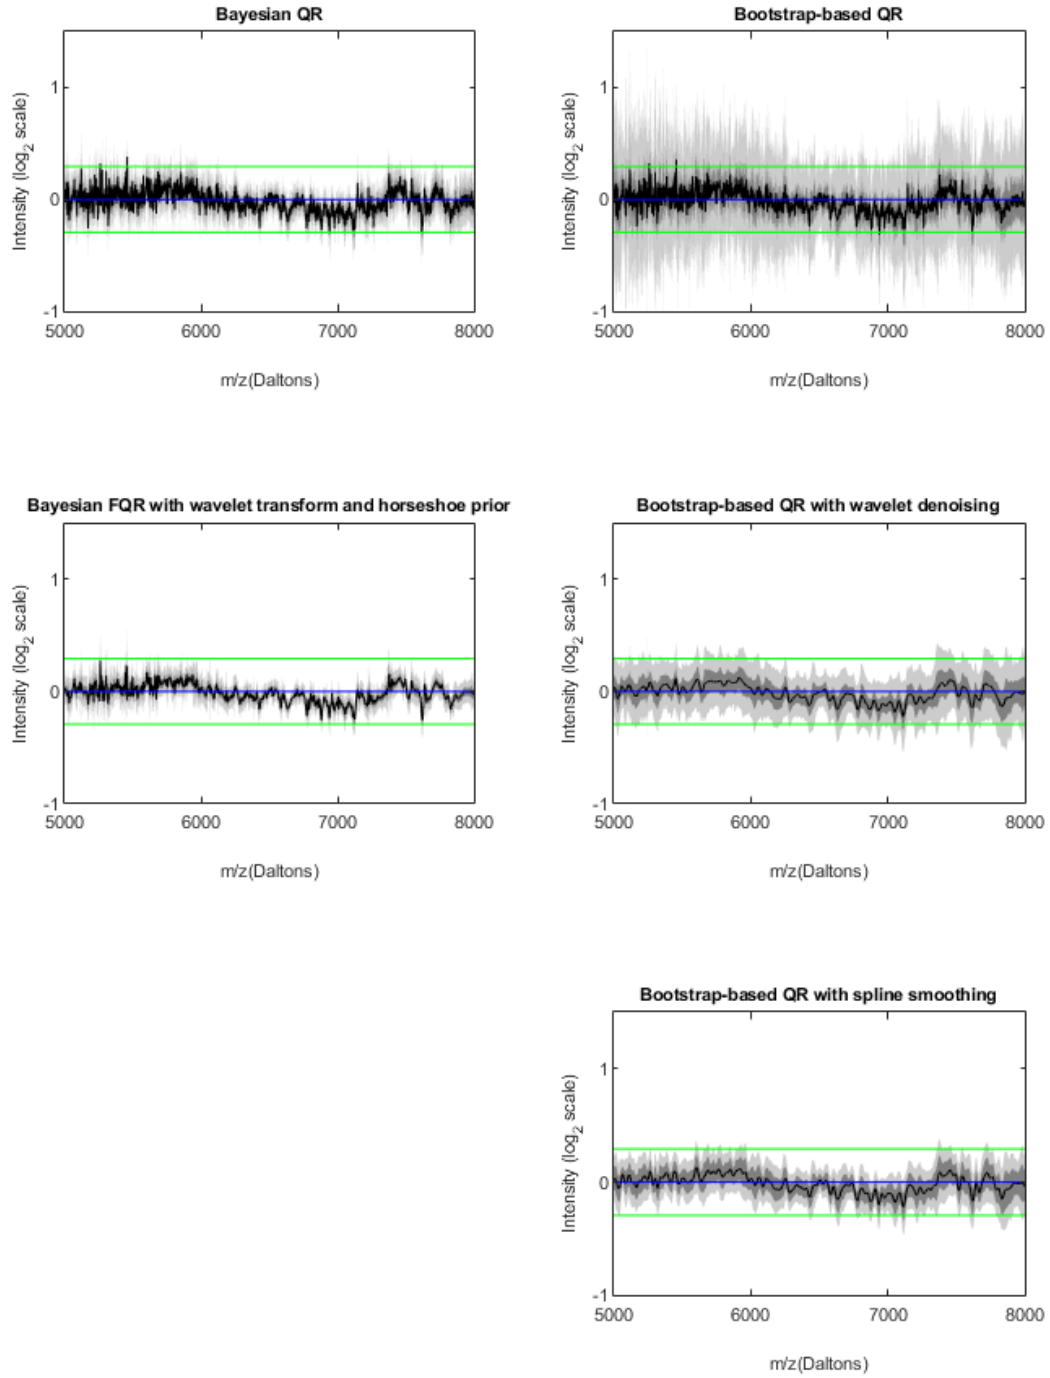

Figure S4(a): Cancer main effect function  $B_2^{0.1}(t)$  in the pancreatic cancer dataset estimated by various methods, with 95% pointwise and simultaneous credible bands.

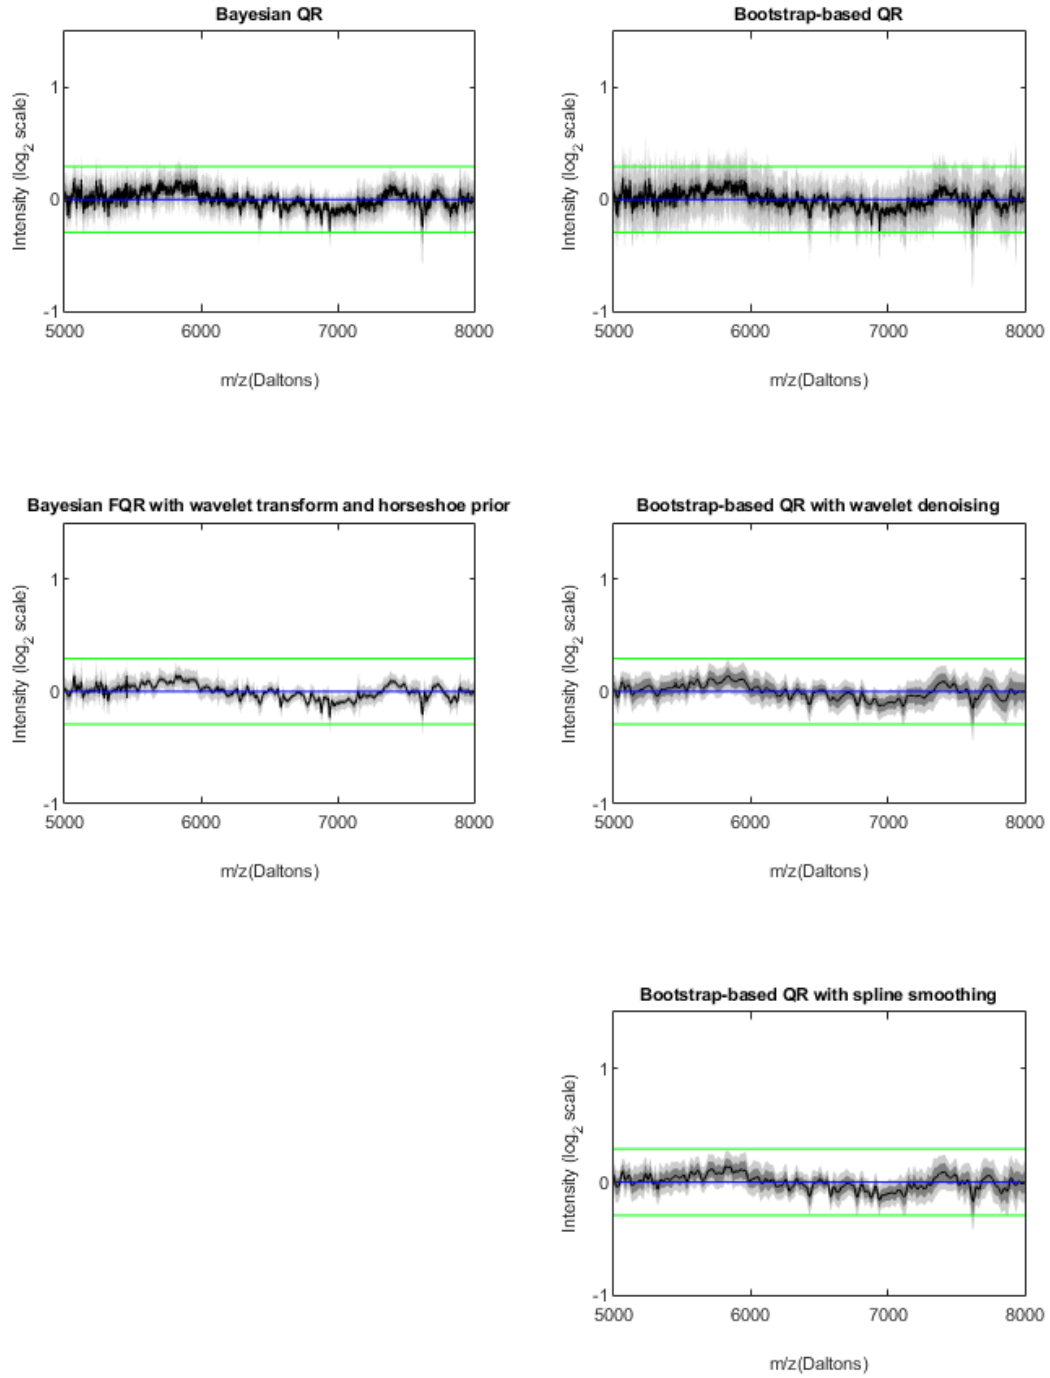

Figure S4(b): Cancer main effect function  $B_2^{0.25}(t)$  in the pancreatic cancer dataset estimated by various methods, with 95% pointwise and simultaneous credible bands.

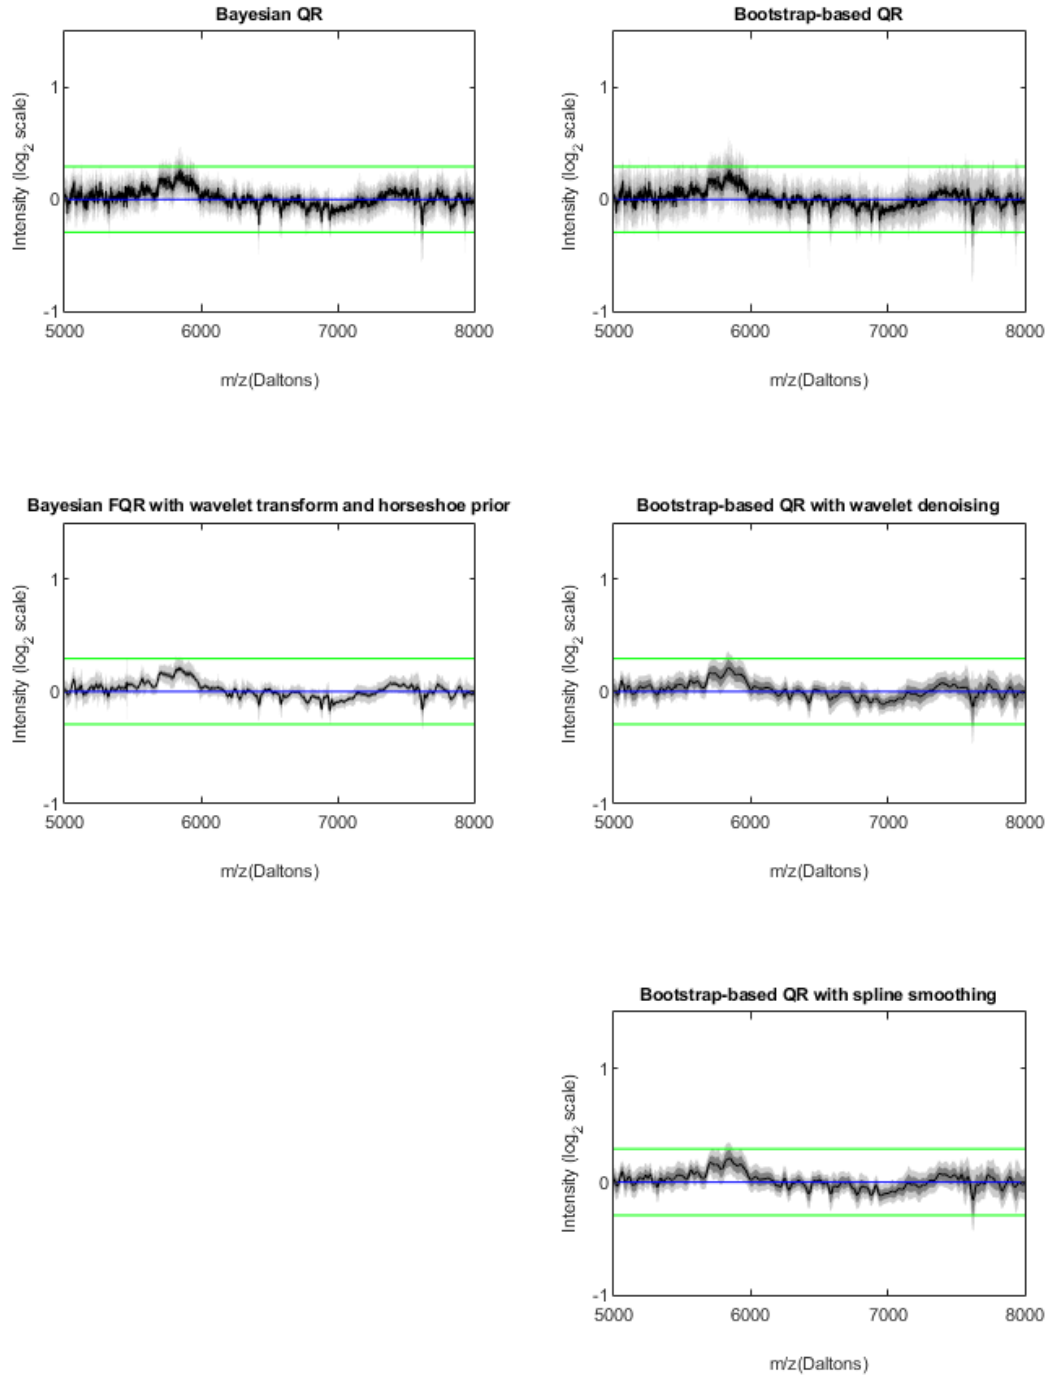

Figure S4(c): Cancer main effect function  $B_2^{0.5}(t)$  in the pancreatic cancer dataset estimated by various methods, with 95% pointwise and simultaneous credible bands.

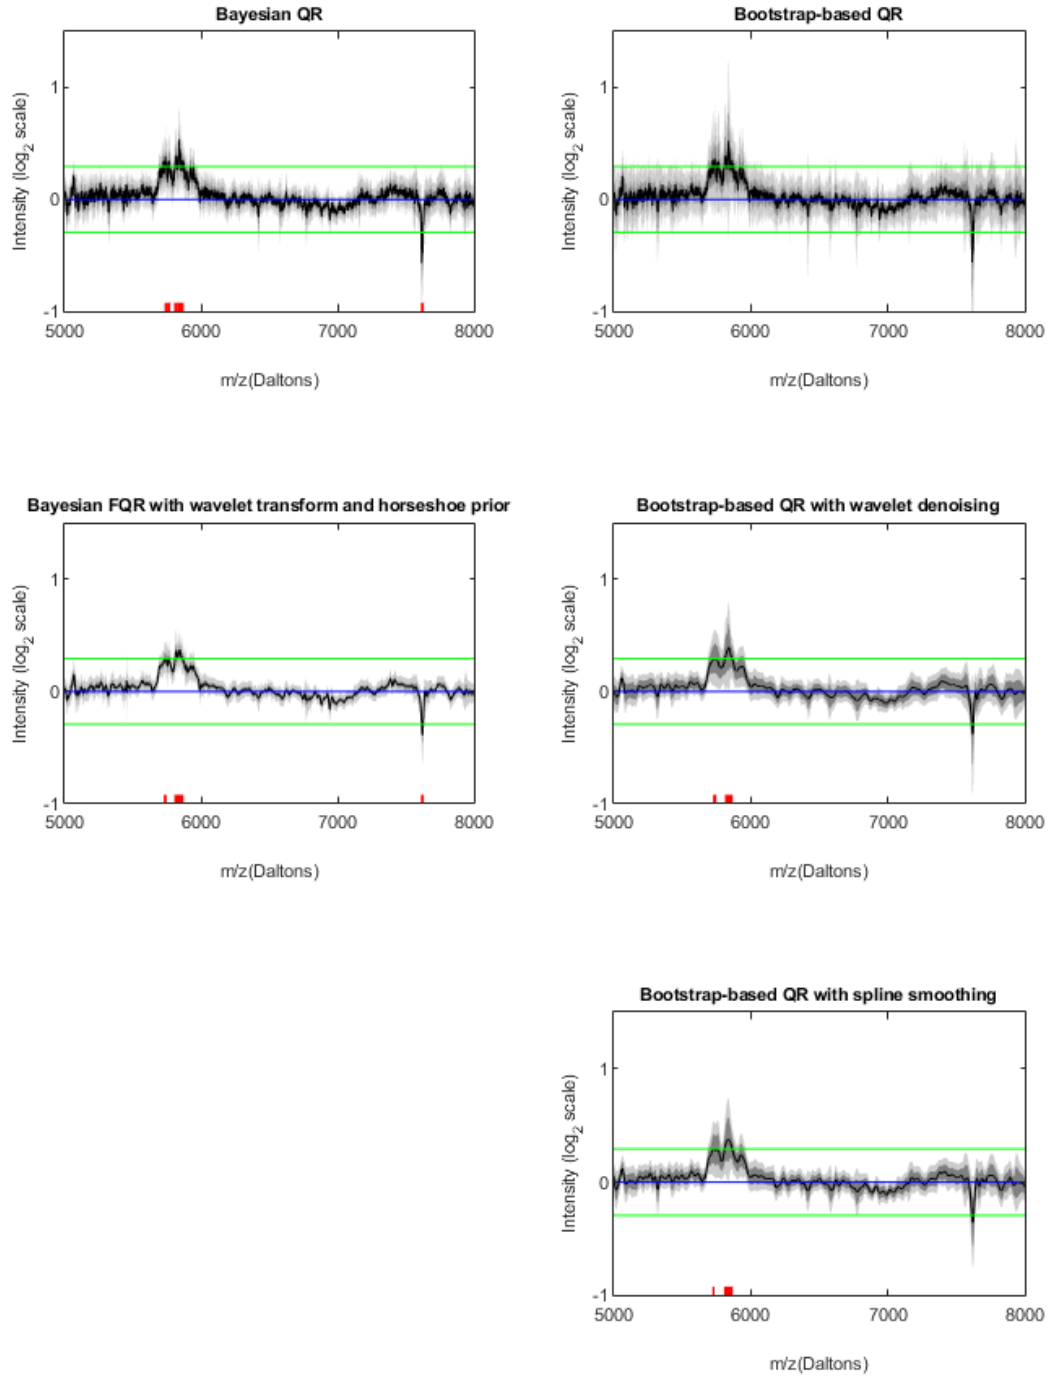

Figure S4(d): Cancer main effect function  $B_2^{0.75}(t)$  in the pancreatic cancer dataset estimated by various methods, with 95% pointwise and simultaneous credible bands. Spectral locations that are flagged as significant are marked on the x-axis.

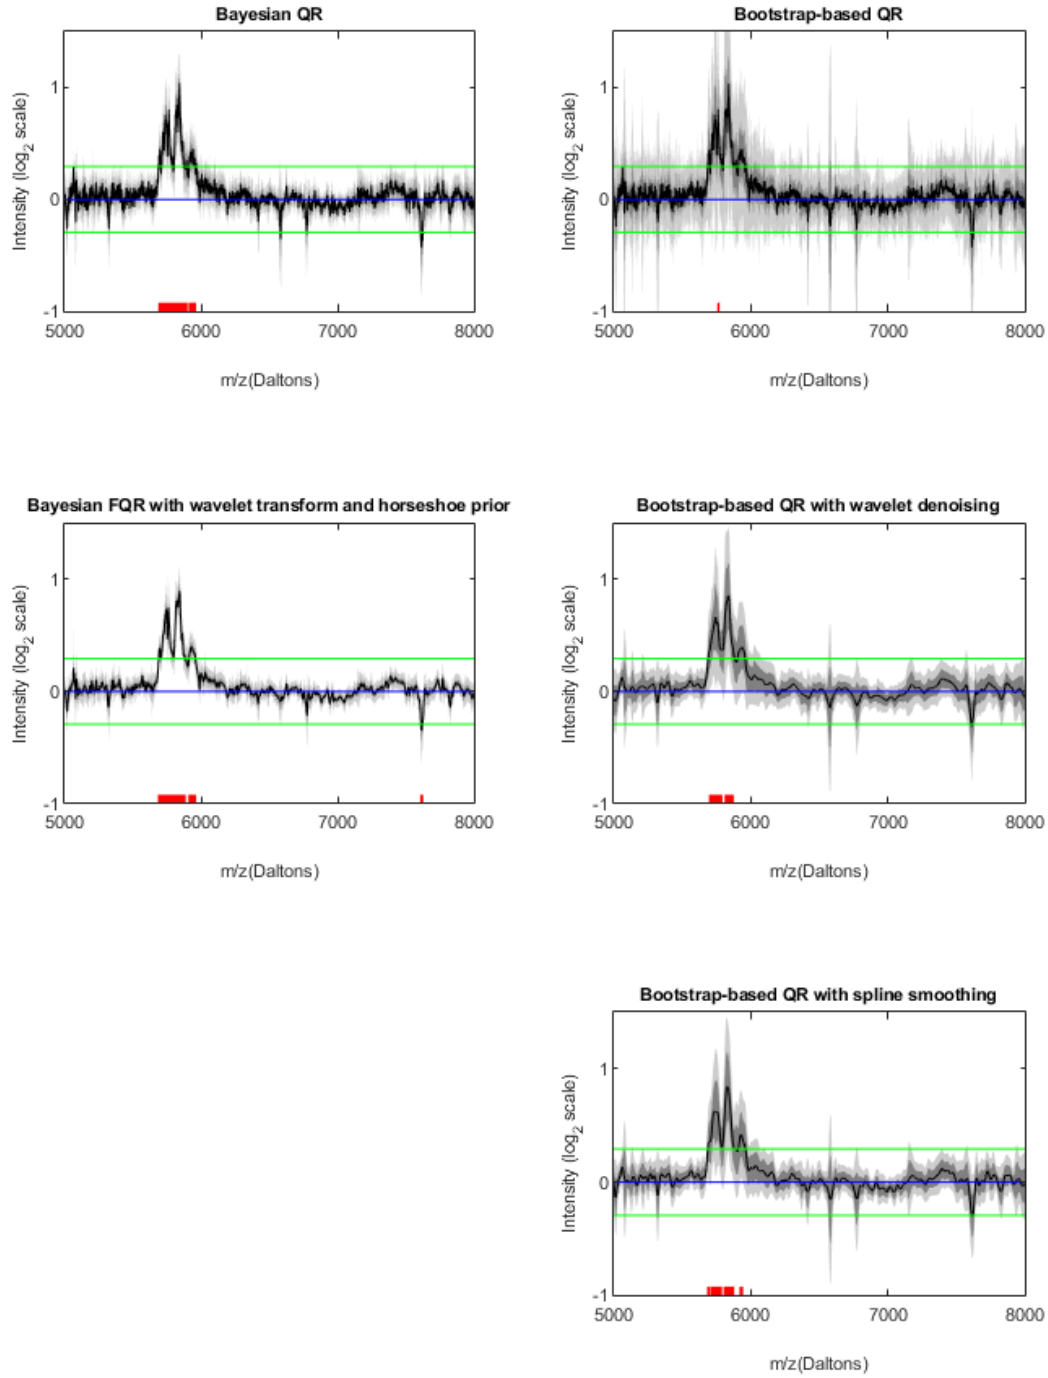

Figure S4(e): Cancer main effect function  $B_2^{0.9}(t)$  in the pancreatic cancer dataset estimated by various methods, with 95% pointwise and simultaneous credible bands. Spectral locations that are flagged as significant are marked on the x-axis.

### 3 Implementation details of FDboost package

We called the R package "FDboost" (Brockhaus and Ruegamer, 2017) to apply the boosting functional regression model proposed by (Brockhaus et al., 2015) to 10 replicate simulation datasets in the right skewed setting to perform FQR for  $\tau = 0.9$ .

A linear base learner with  $df = 1$  was specified for the group effect covariate, and a smooth P-spline base learner with  $df = 20$  was specified for the non-linear effect in  $t$  direction. A composed basis was constructed by combining these two base learners using the  $\otimes$  operator, so that only the marginal basis in  $t$  direction was regularized by a L2 penalty. Model estimation was performed by component-wise gradient boosting. As recommended by the authors, we determined the optimal number of boosting iterations from a search grid of 1 to 2000 by cross validation while fixing the step-length  $\nu = 0.2$ . For each replicate dataset, we found that the point estimate of the group main effect function  $B_2^{0.9}(t)$  based on the model fit corresponding to the optimal number of boosting iterations was identically 0, and this process took 10 minutes on a 64-bit operating system with 2 processors and an RAM of 256GB.

We then repeated the model fitting and tuning process above with different specifications, which are manually chosen to be more appropriate for spiky and spatially heterogeneous functional data. Specifically, we used 150 knots, 1st order regression spline, and ridge penalty for the base learner modeling non-linear effect in  $t$  direction. This time we were able to get a reasonable but very noisy point estimate of  $B_2^{0.9}(t)$ .

## References

- Bhattacharya, A., D. Pati, N. S. Pillai, and D. B. Dunson (2015). Dirichlet–laplace priors for optimal shrinkage. *Journal of the American Statistical Association* 110(512), 1479–1490.
- Brockhaus, S. and D. Ruegamer (2017). *FDboost: Boosting Functional Regression Models*.
- Brockhaus, S., F. Scheipl, T. Hothorn, and S. Greven (2015). The functional linear array model. *Statistical Modelling* 15(3), 279–300.

- Carvalho, C. M., N. G. Polson, and J. G. Scott (2009). Handling sparsity via the horseshoe. In *Artificial Intelligence and Statistics*, pp. 73–80.
- Griffin, J. E., P. J. Brown, et al. (2010). Inference with normal-gamma prior distributions in regression problems. *Bayesian Analysis* 5(1), 171–188.
- Makalic, E. and D. F. Schmidt (2016). A simple sampler for the horseshoe estimator. *IEEE Signal Processing Letters* 23(1), 179–182.
